# Supplementary material for: Scenario-Transferable Semantic Graph Reasoning for Interaction-Aware Probabilistic Prediction
Source: arXiv:2004.03053 source file (2022-11-14)
Supplement: Supplementary file 1 [file appendix.tex]

\appendices{
\section{Theoretical Proof}
\subsection{Proof for Theorem 1}

\subsection{Proof for Theorem 2 (Number of aggregators needed)}

\subsection{Proof for Theorem 3 (Injective functions on countable multisets)}

\section{Demonstration}
}
